# Supplementary material for: Detail Enhanced Gaussian Splatting for Large-Scale Volumetric Capture
Source: arXiv:2511.21697 source file (2025-10-31)
Supplement: Supplementary file 1 [file add_results.tex]

\setcounter{figure}{3}
\begin{figure*}
\centering
\begin{tabular}{cc}
     Our 4DGS reconstruction & Our Detail Enhanced Results  \\

    \begin{minipage}{0.5\linewidth}
    \centering
    \adjincludegraphics[trim= {0.\width} {0.0\height} {0.\width} {0.0\height}, clip, clip, width=\linewidth]{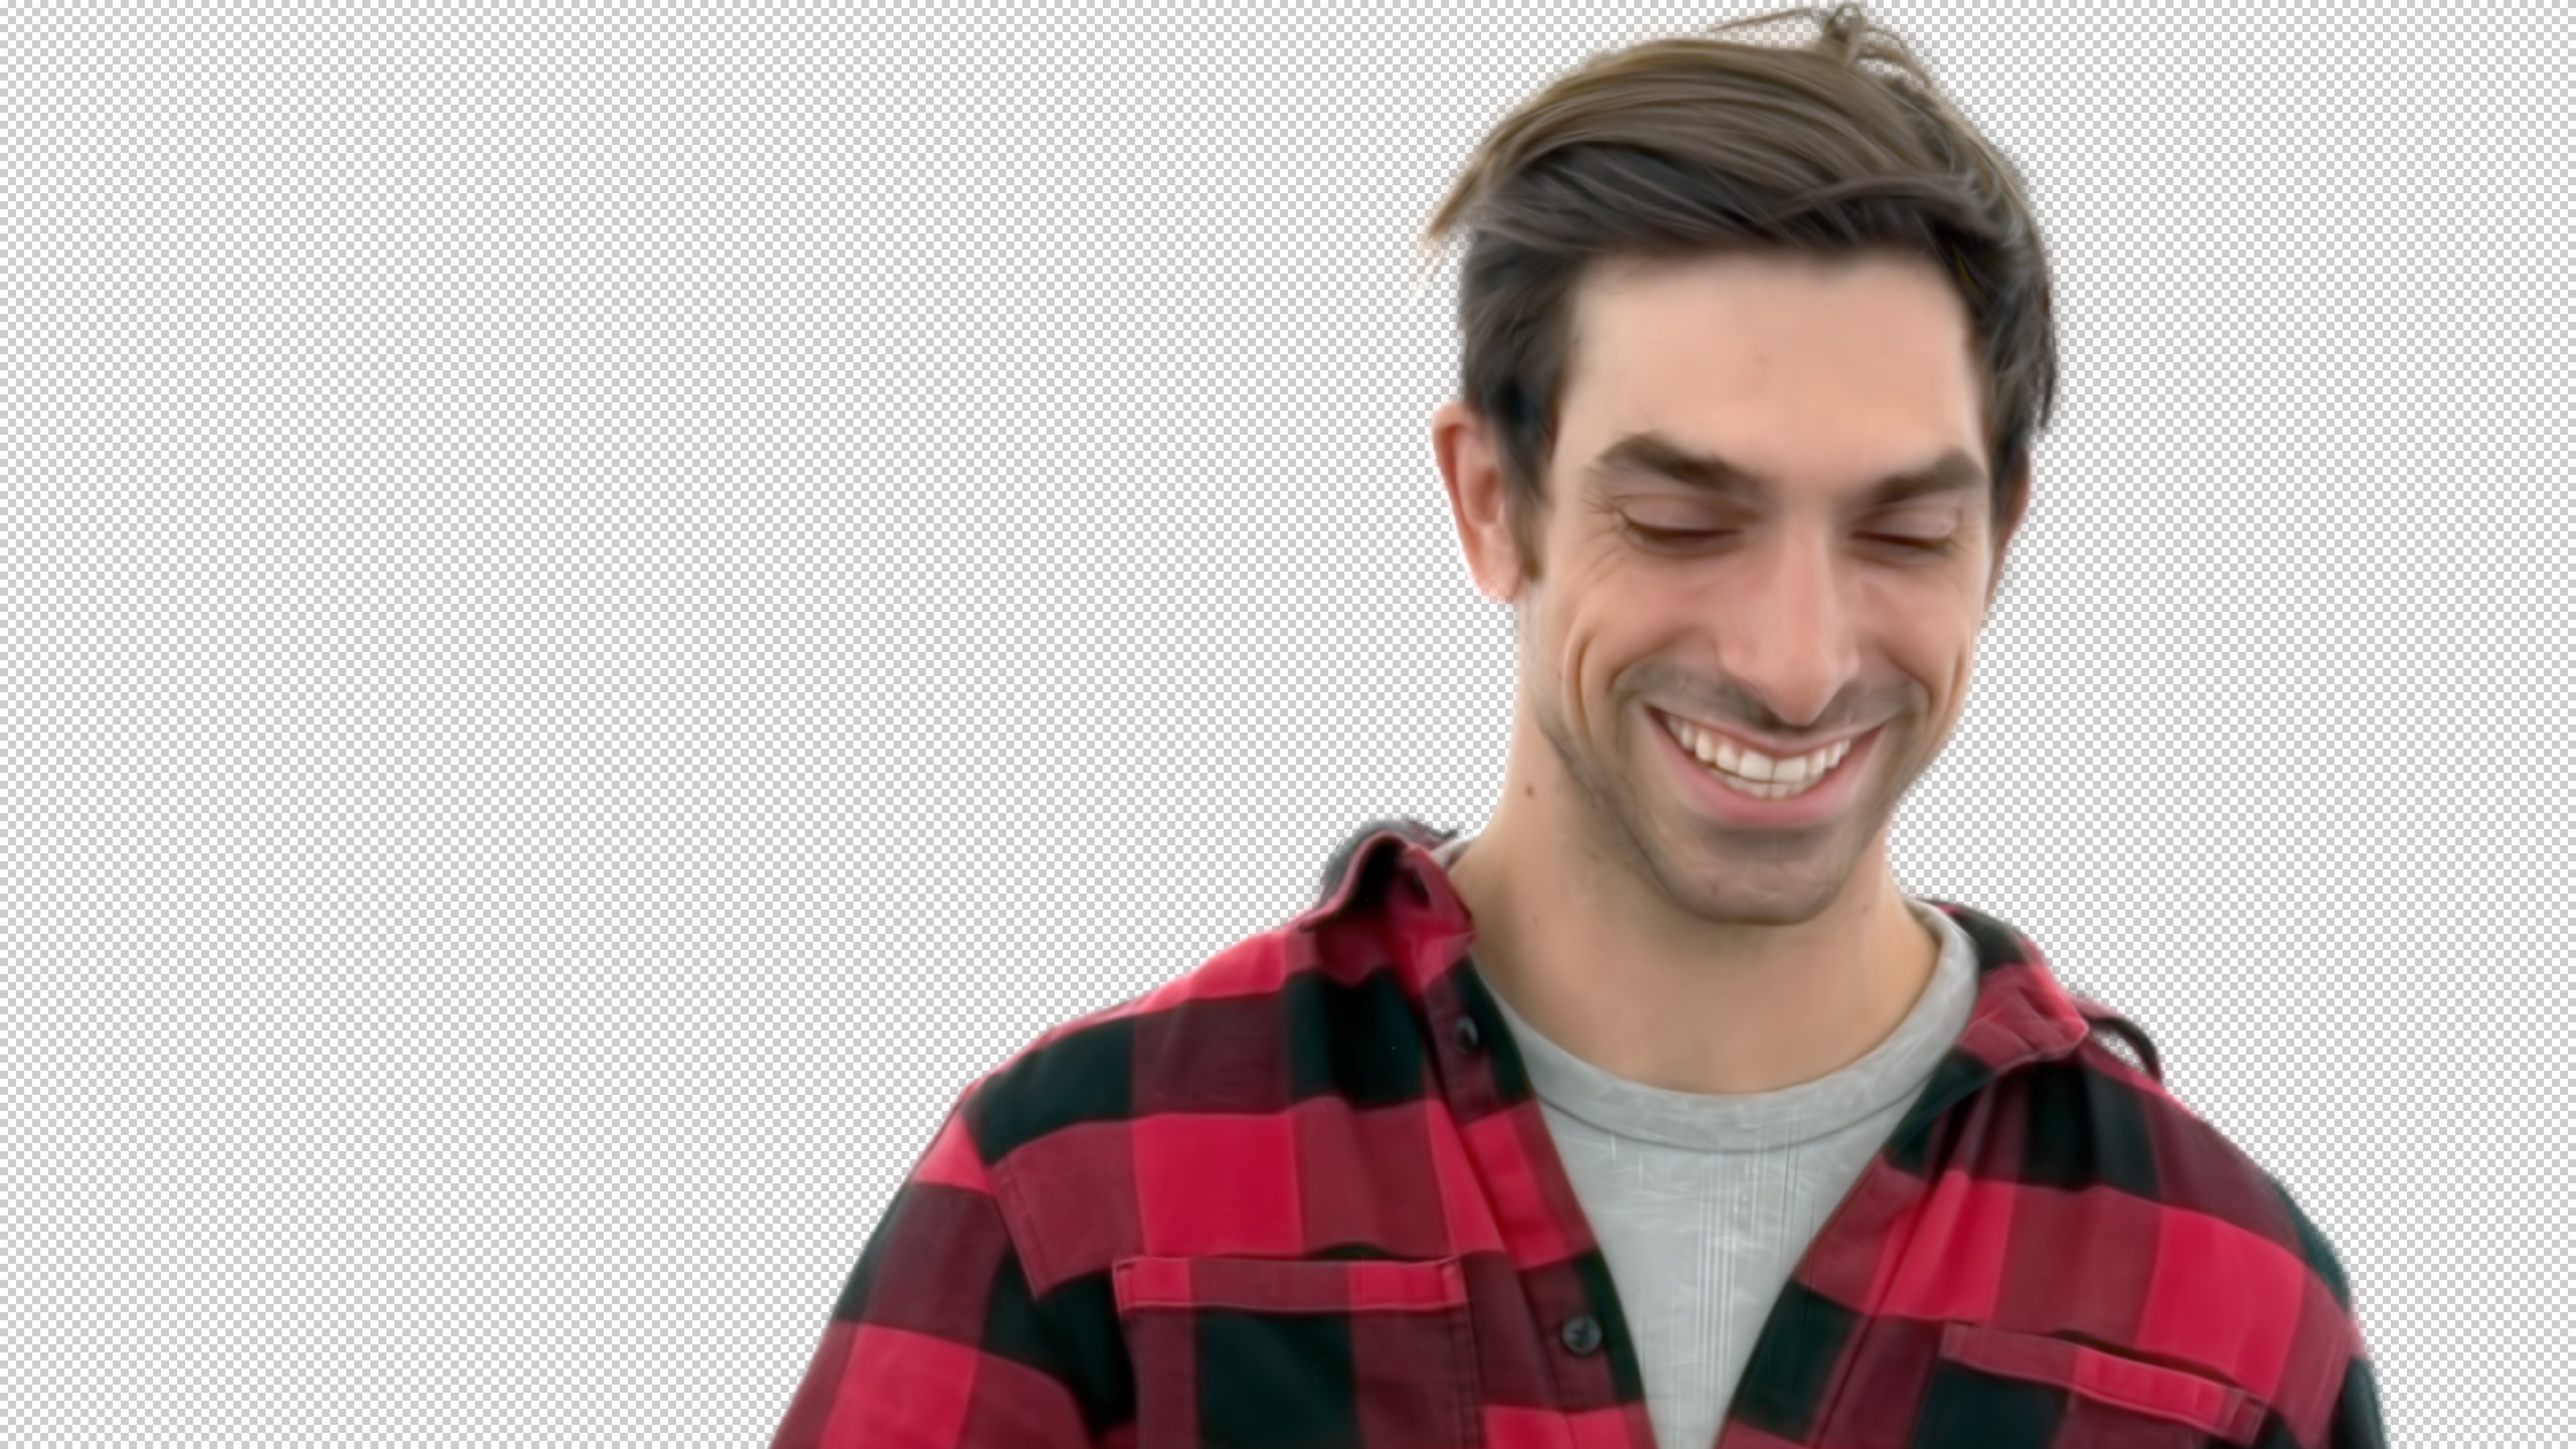}
    \\
    \adjincludegraphics[trim= {0.5\width} {0.4\height} {0.2\width} {0.3\height}, clip, width=\linewidth]{images/main_results/supp/input/cam0000_1041.jpg}
    \end{minipage}

&
    
    \begin{minipage}{0.5\linewidth}
    \centering
    \adjincludegraphics[trim= {0.\width} {0.0\height} {0.\width} {0.0\height}, clip, clip, width=\linewidth]{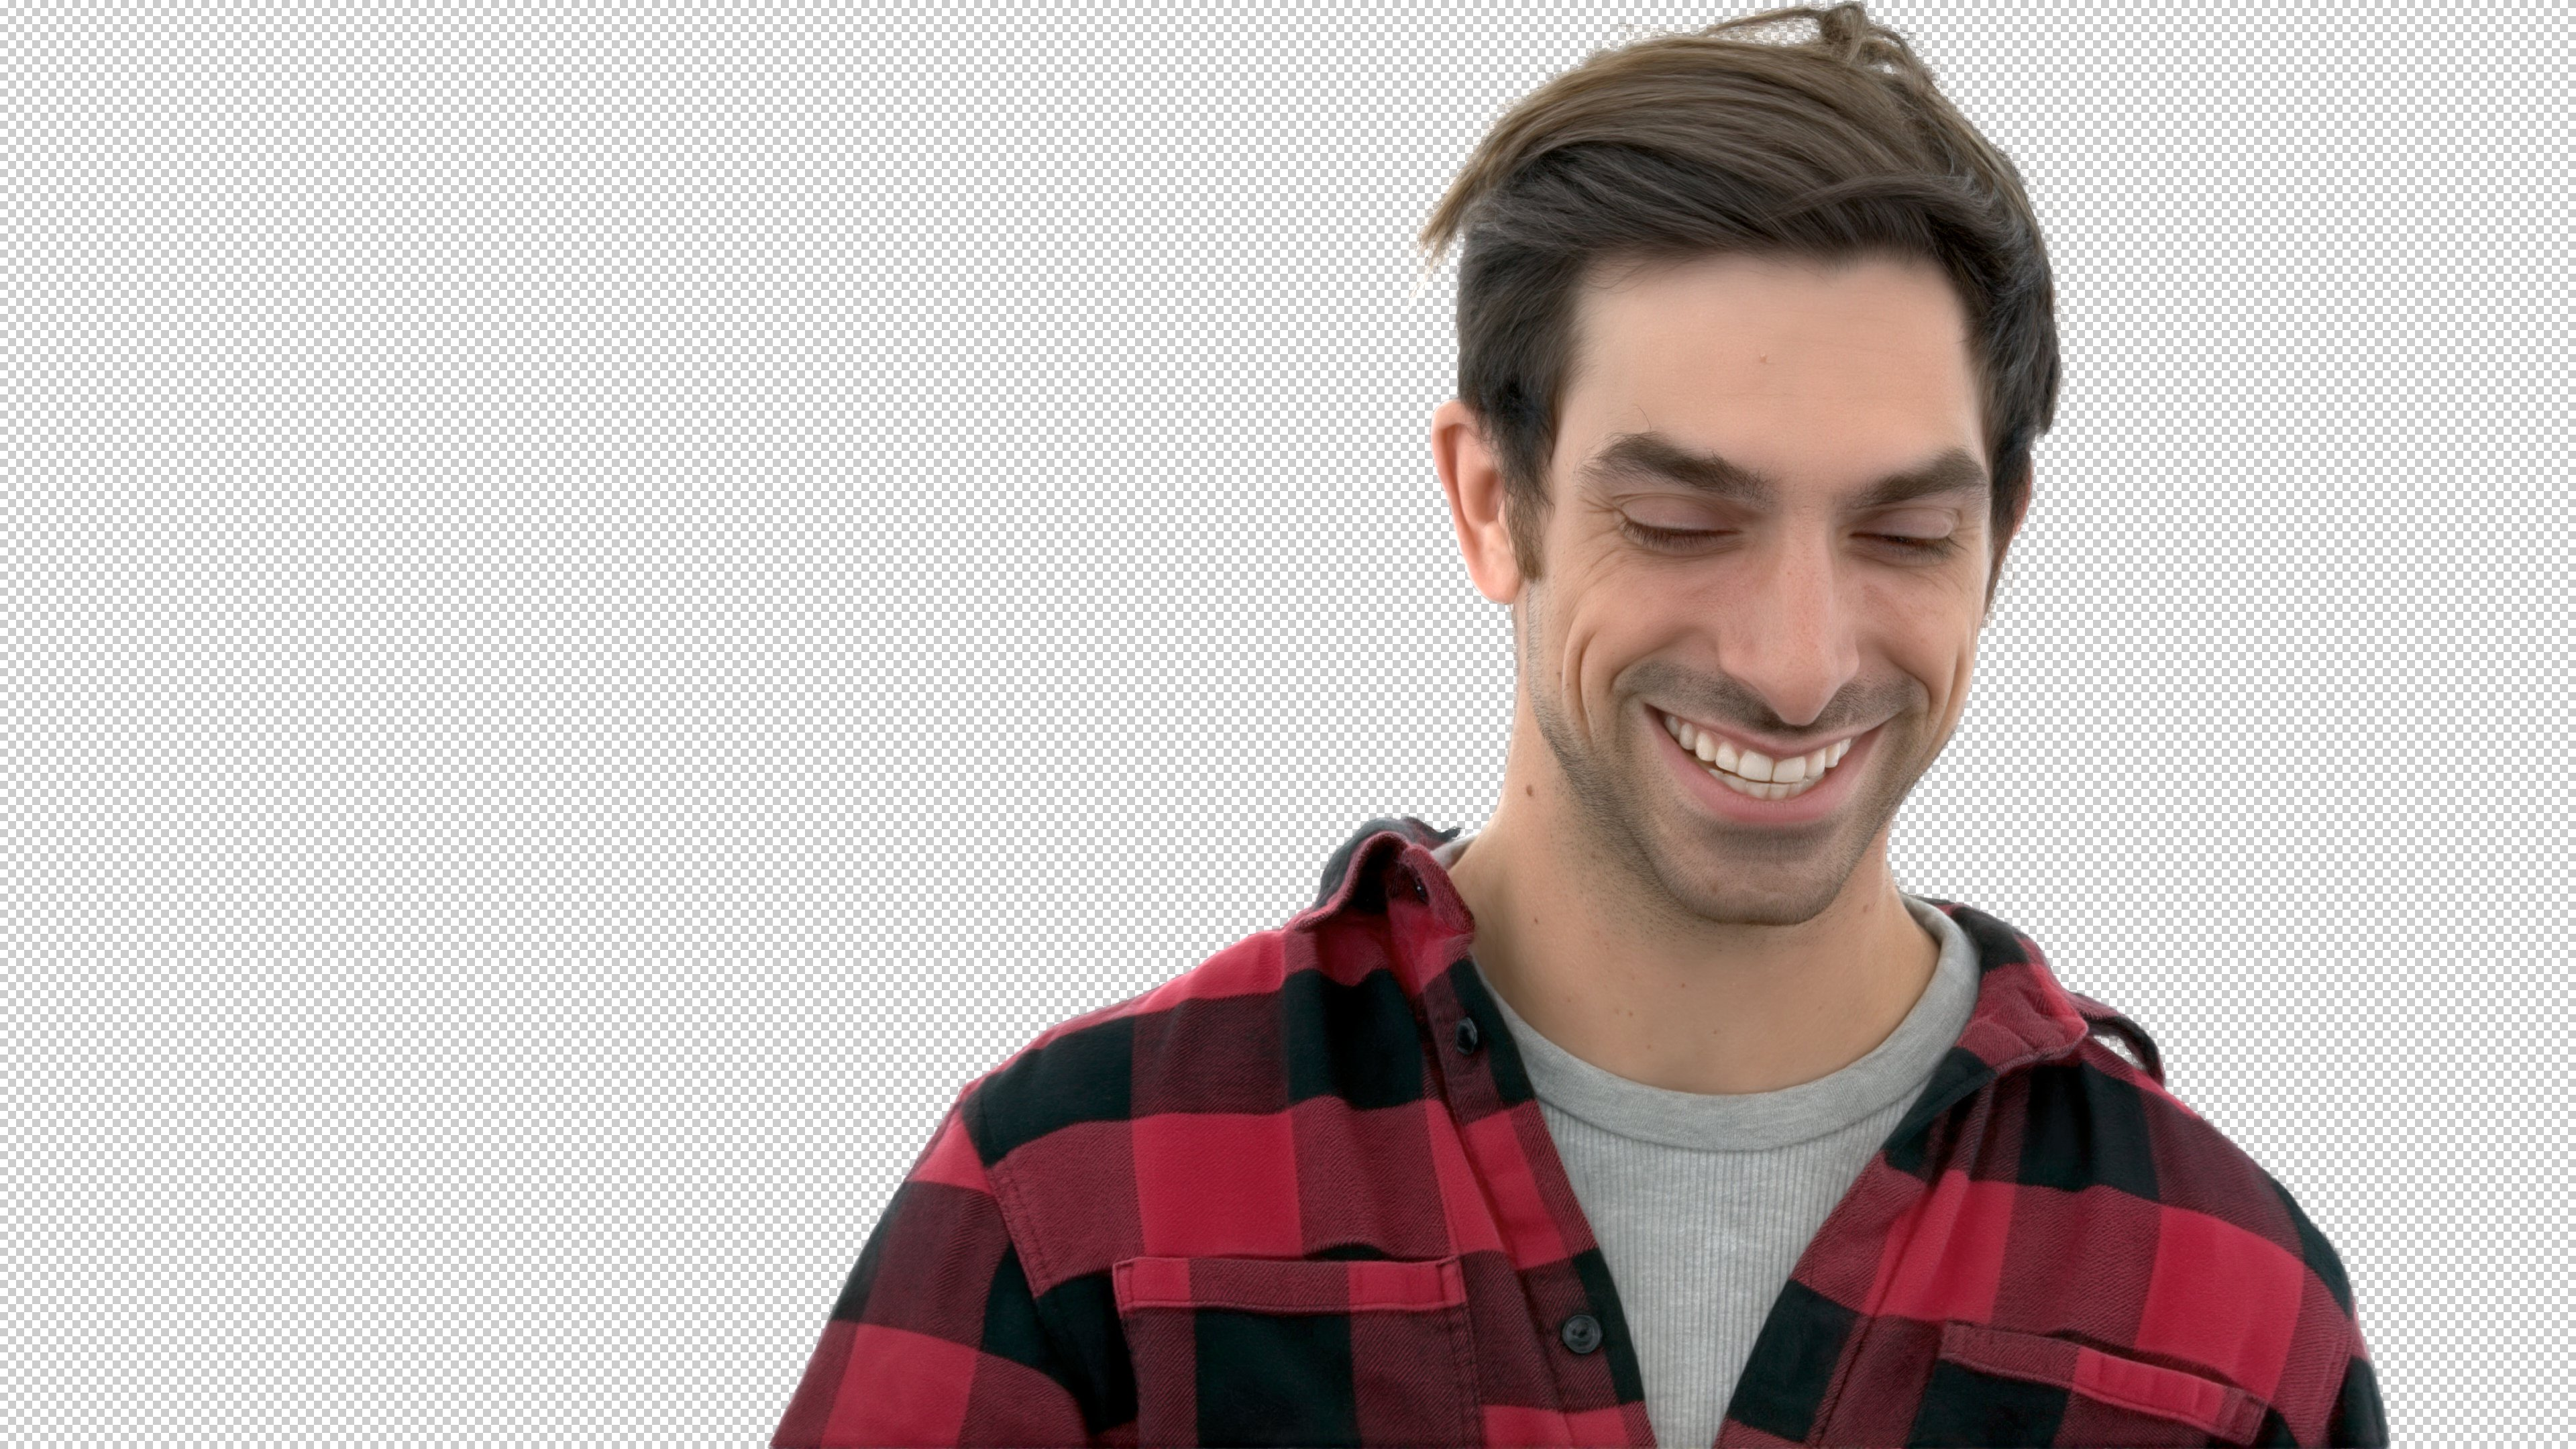}
    \\
    \adjincludegraphics[trim= {0.5\width} {0.4\height} {0.2\width} {0.3\height}, clip, width=\linewidth]{images/main_results/supp/output/cam0000_1041.jpg}
    \end{minipage} \\

    \noalign{\vskip 1mm}

    \begin{minipage}{0.5\linewidth}
    \centering
    \adjincludegraphics[trim= {0.\width} {0.0\height} {0.\width} {0.0\height}, clip, clip, width=\linewidth]{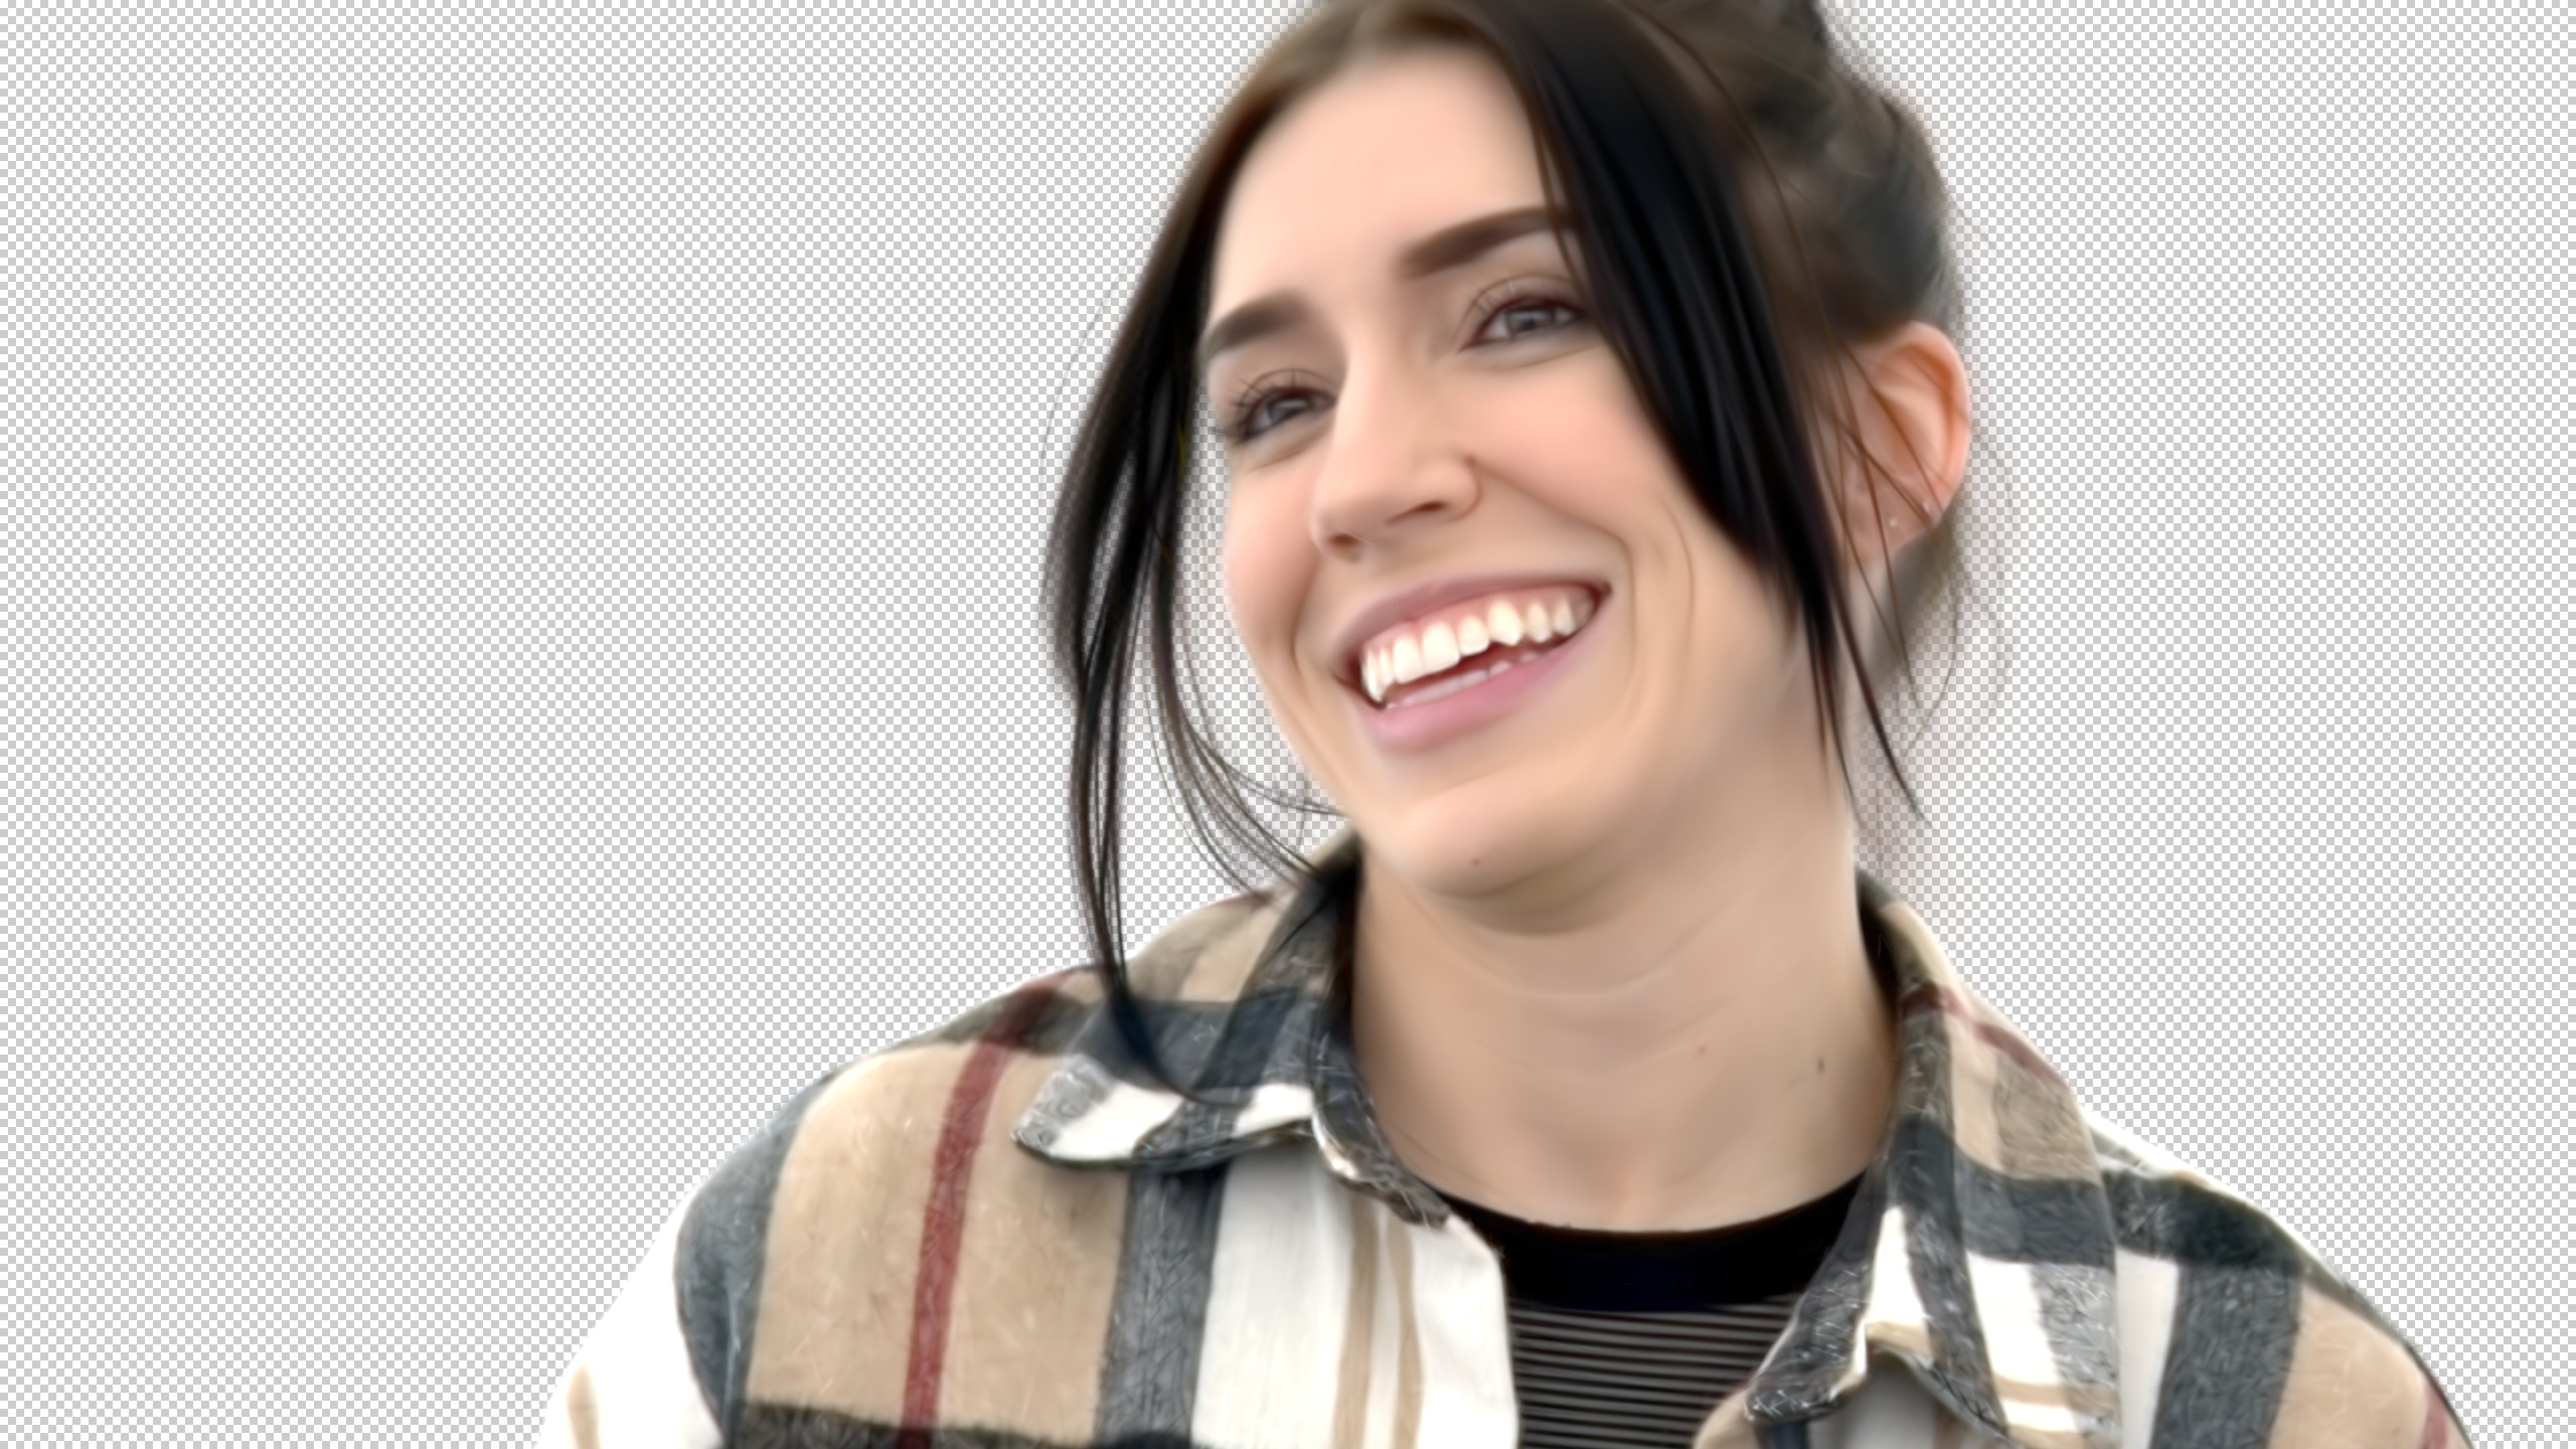}
    \\
    \adjincludegraphics[trim= {0.35\width} {0.4\height} {0.25\width} {0.2\height}, clip, width=\linewidth]{images/main_results/supp/input/cam0000_1066.jpg}
    \end{minipage}

&
    
    \begin{minipage}{0.5\linewidth}
    \centering
    \adjincludegraphics[trim= {0.\width} {0.0\height} {0.\width} {0.0\height}, clip, clip, width=\linewidth]{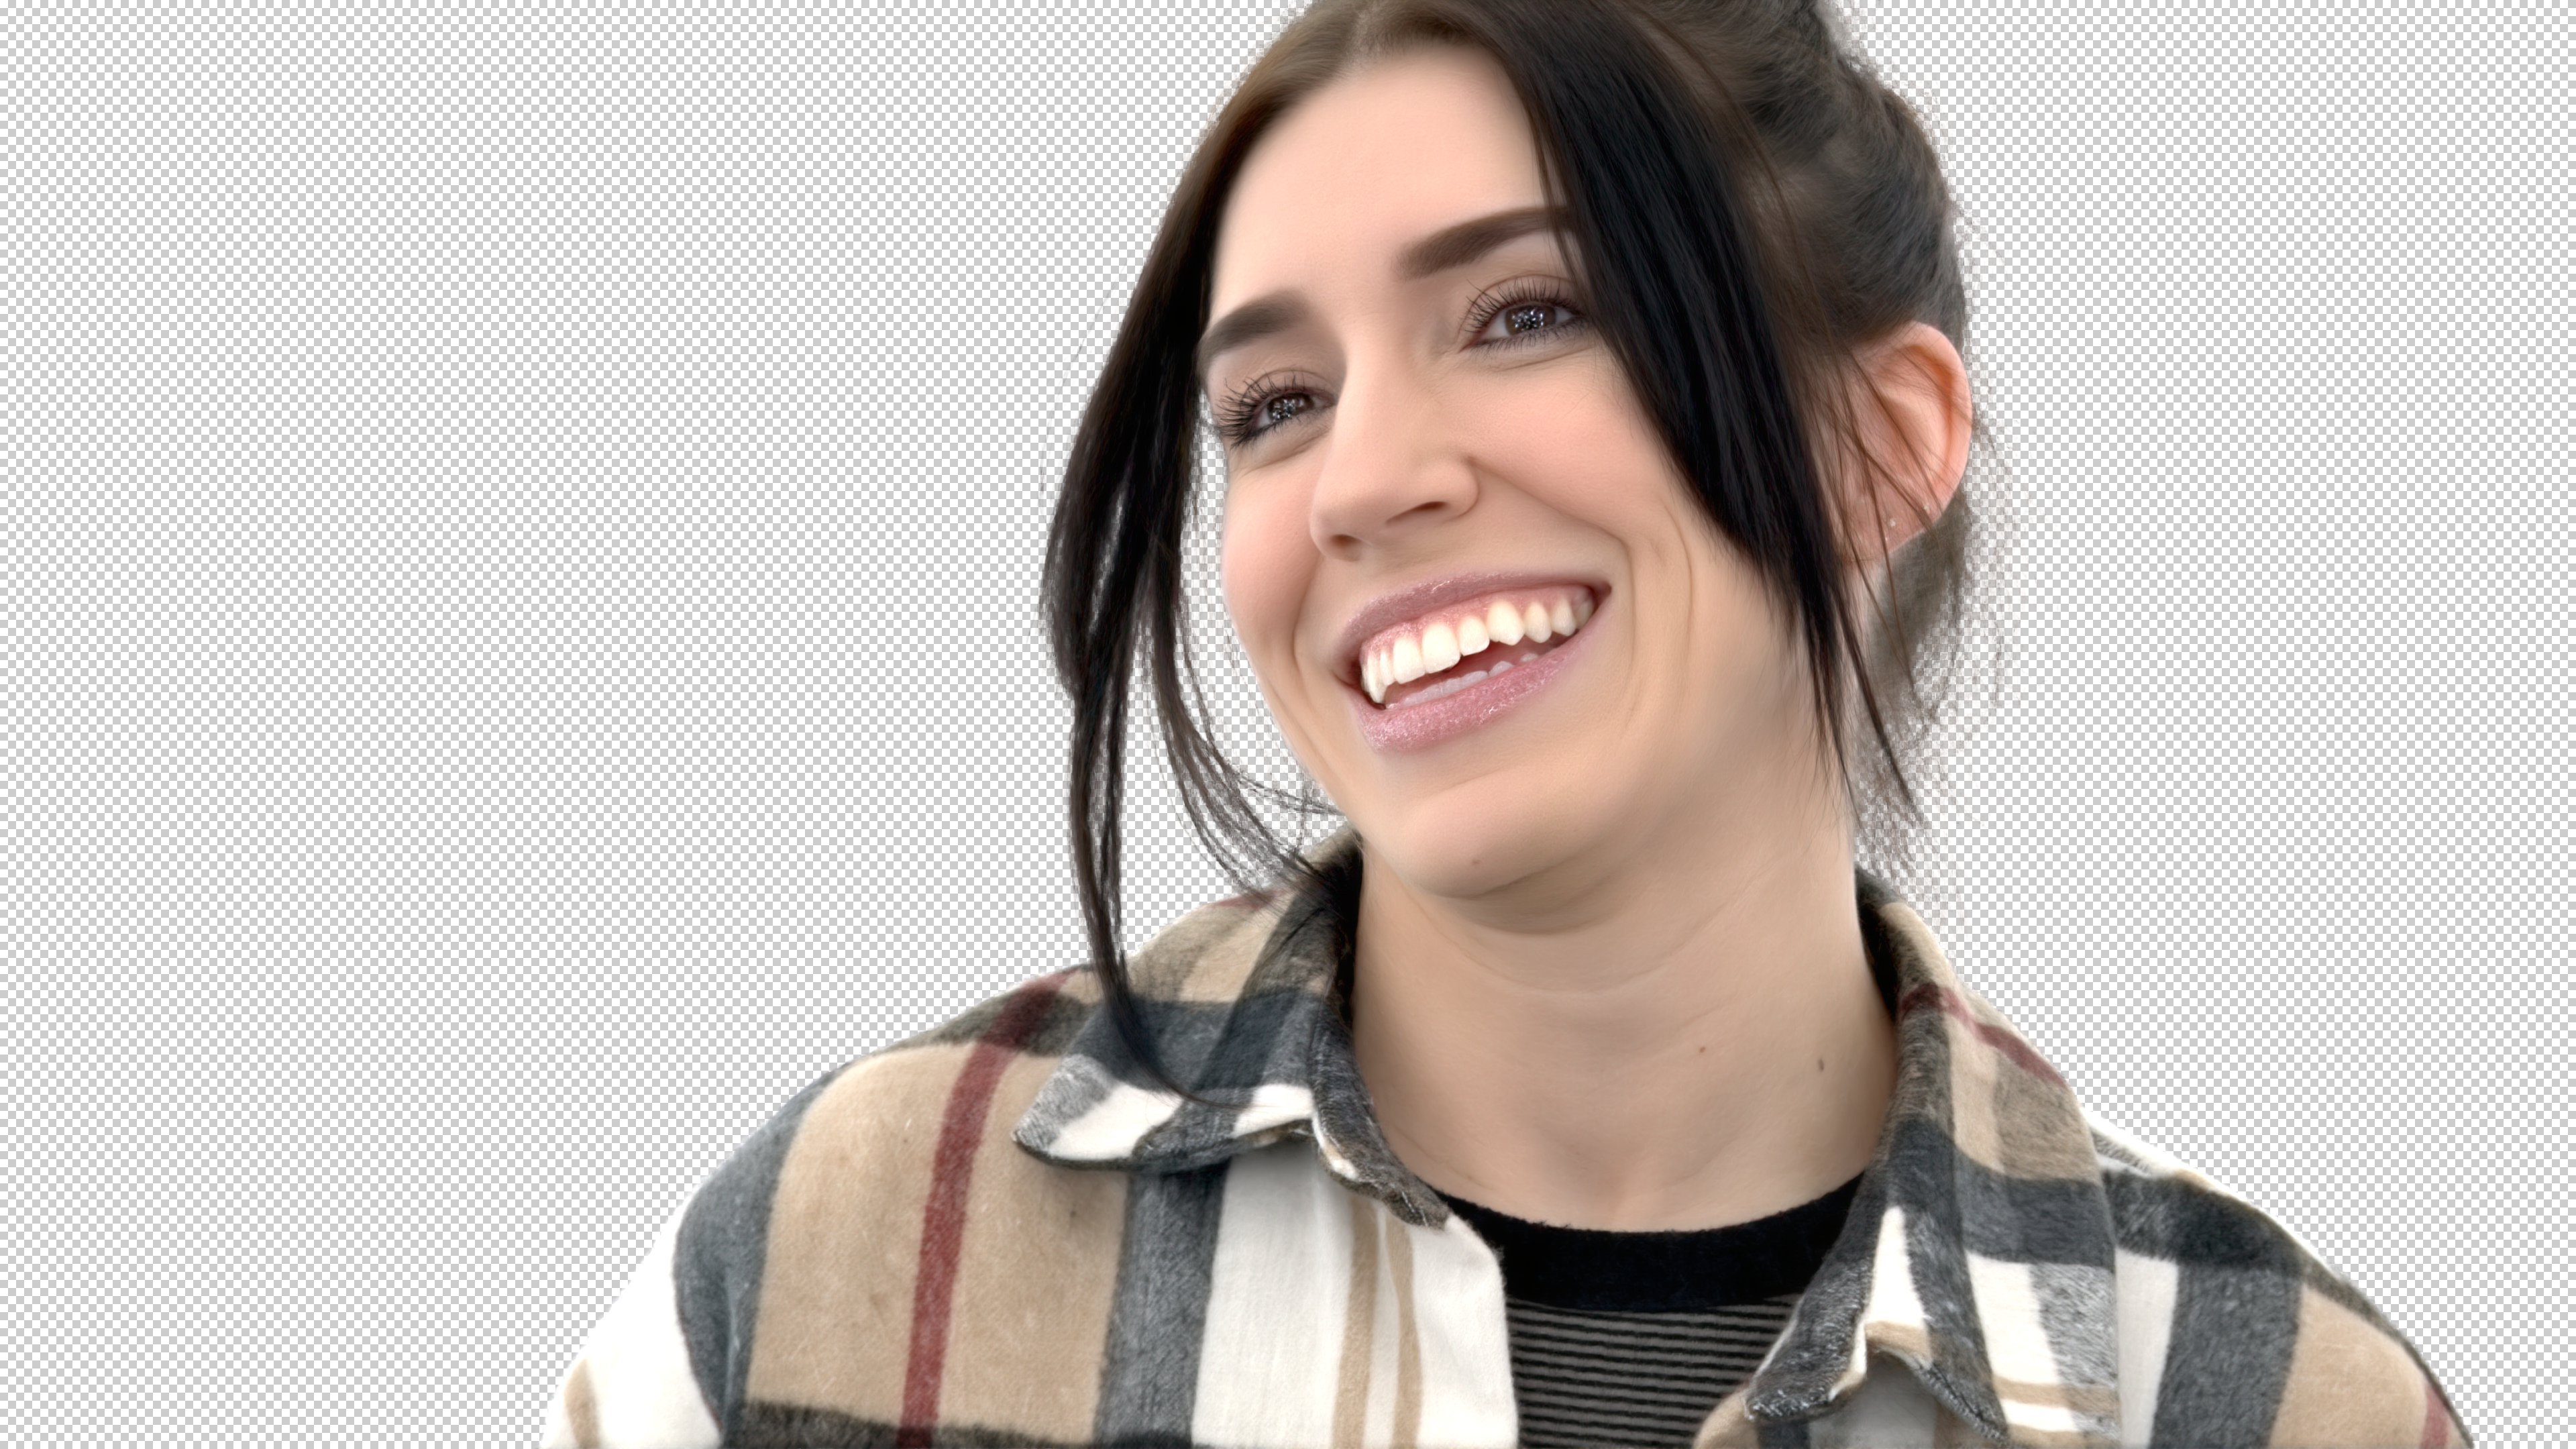}
    \\
    \adjincludegraphics[trim= {0.35\width} {0.4\height} {0.25\width} {0.2\height}, clip, width=\linewidth]{images/main_results/supp/output/cam0000_1066.jpg}
    \end{minipage} \\

\end{tabular}
\end{figure*}
\begin{figure*}\ContinuedFloat
    \begin{tabular}{cc}  

    \begin{minipage}{0.5\linewidth}
    \centering
    \adjincludegraphics[trim= {0.\width} {0.0\height} {0.\width} {0.0\height}, clip, clip, width=\linewidth]{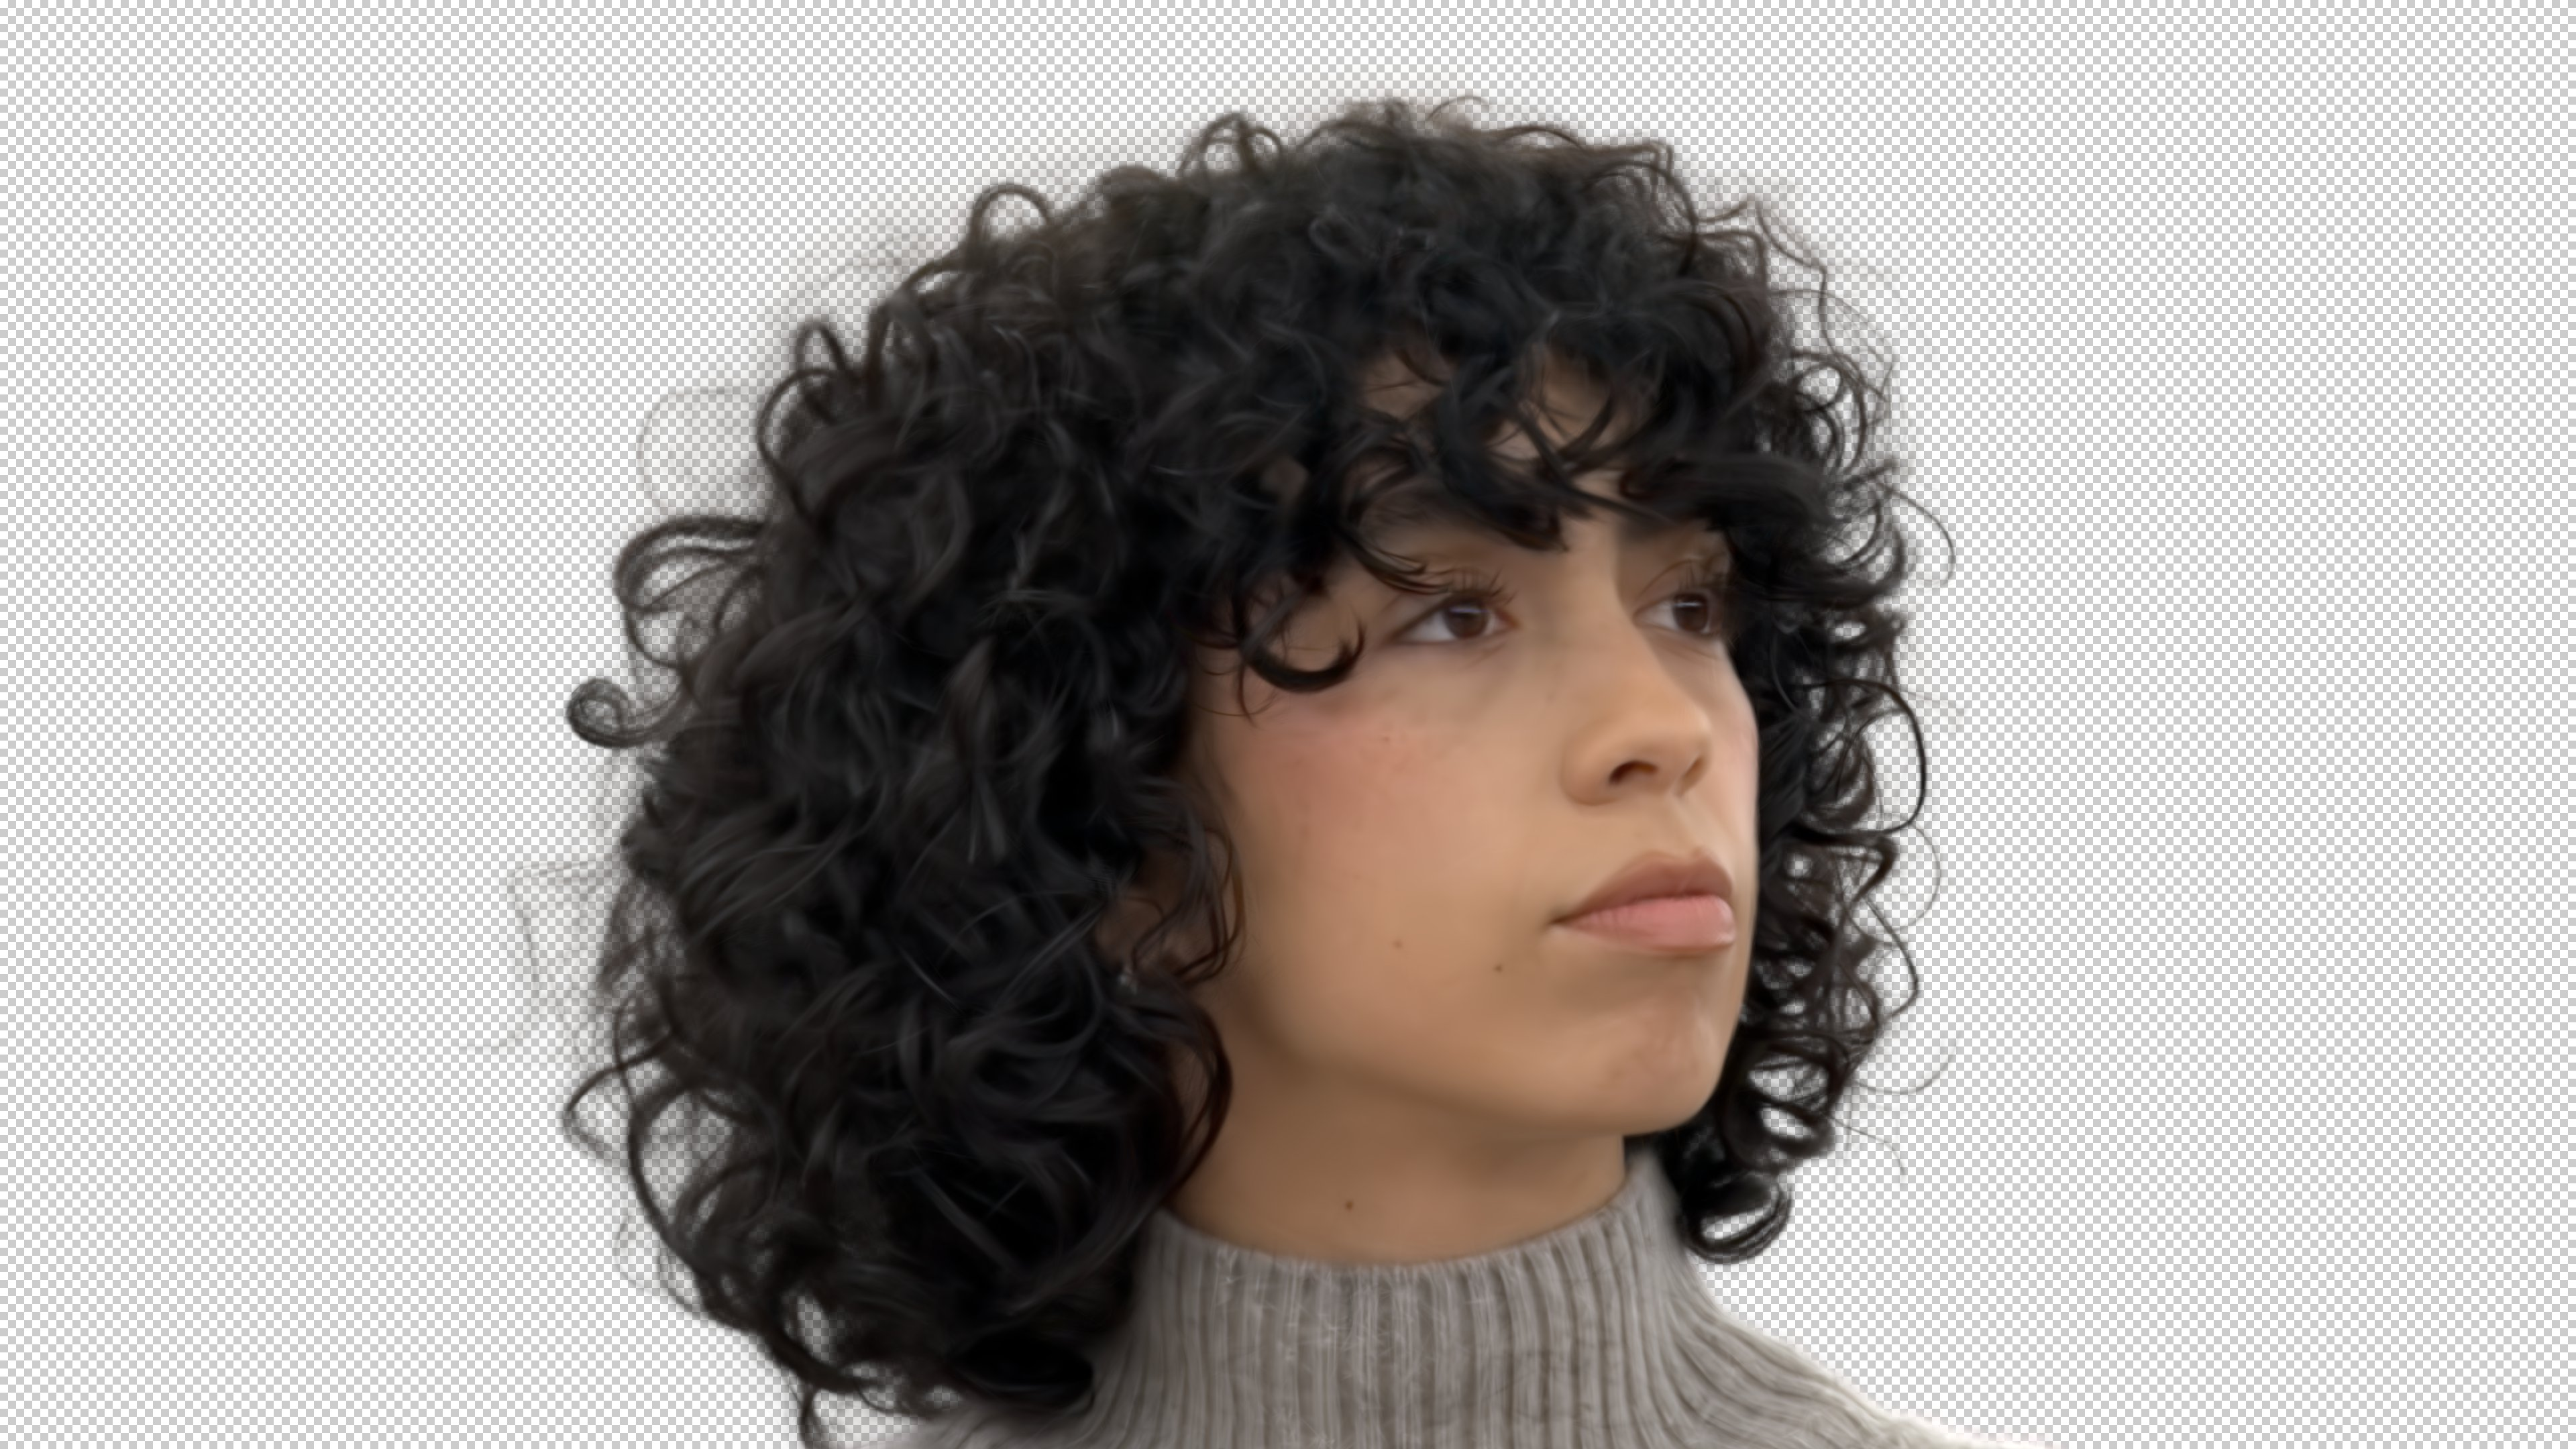}
    \\
    \adjincludegraphics[trim= {0.3\width} {0.3\height} {0.3\width} {0.3\height}, clip, width=\linewidth]{images/main_results/supp/input/cam0000_1114.jpg}
    \end{minipage}

&
    
    \begin{minipage}{0.5\linewidth}
    \centering
    \adjincludegraphics[trim= {0.\width} {0.0\height} {0.\width} {0.0\height}, clip, clip, width=\linewidth]{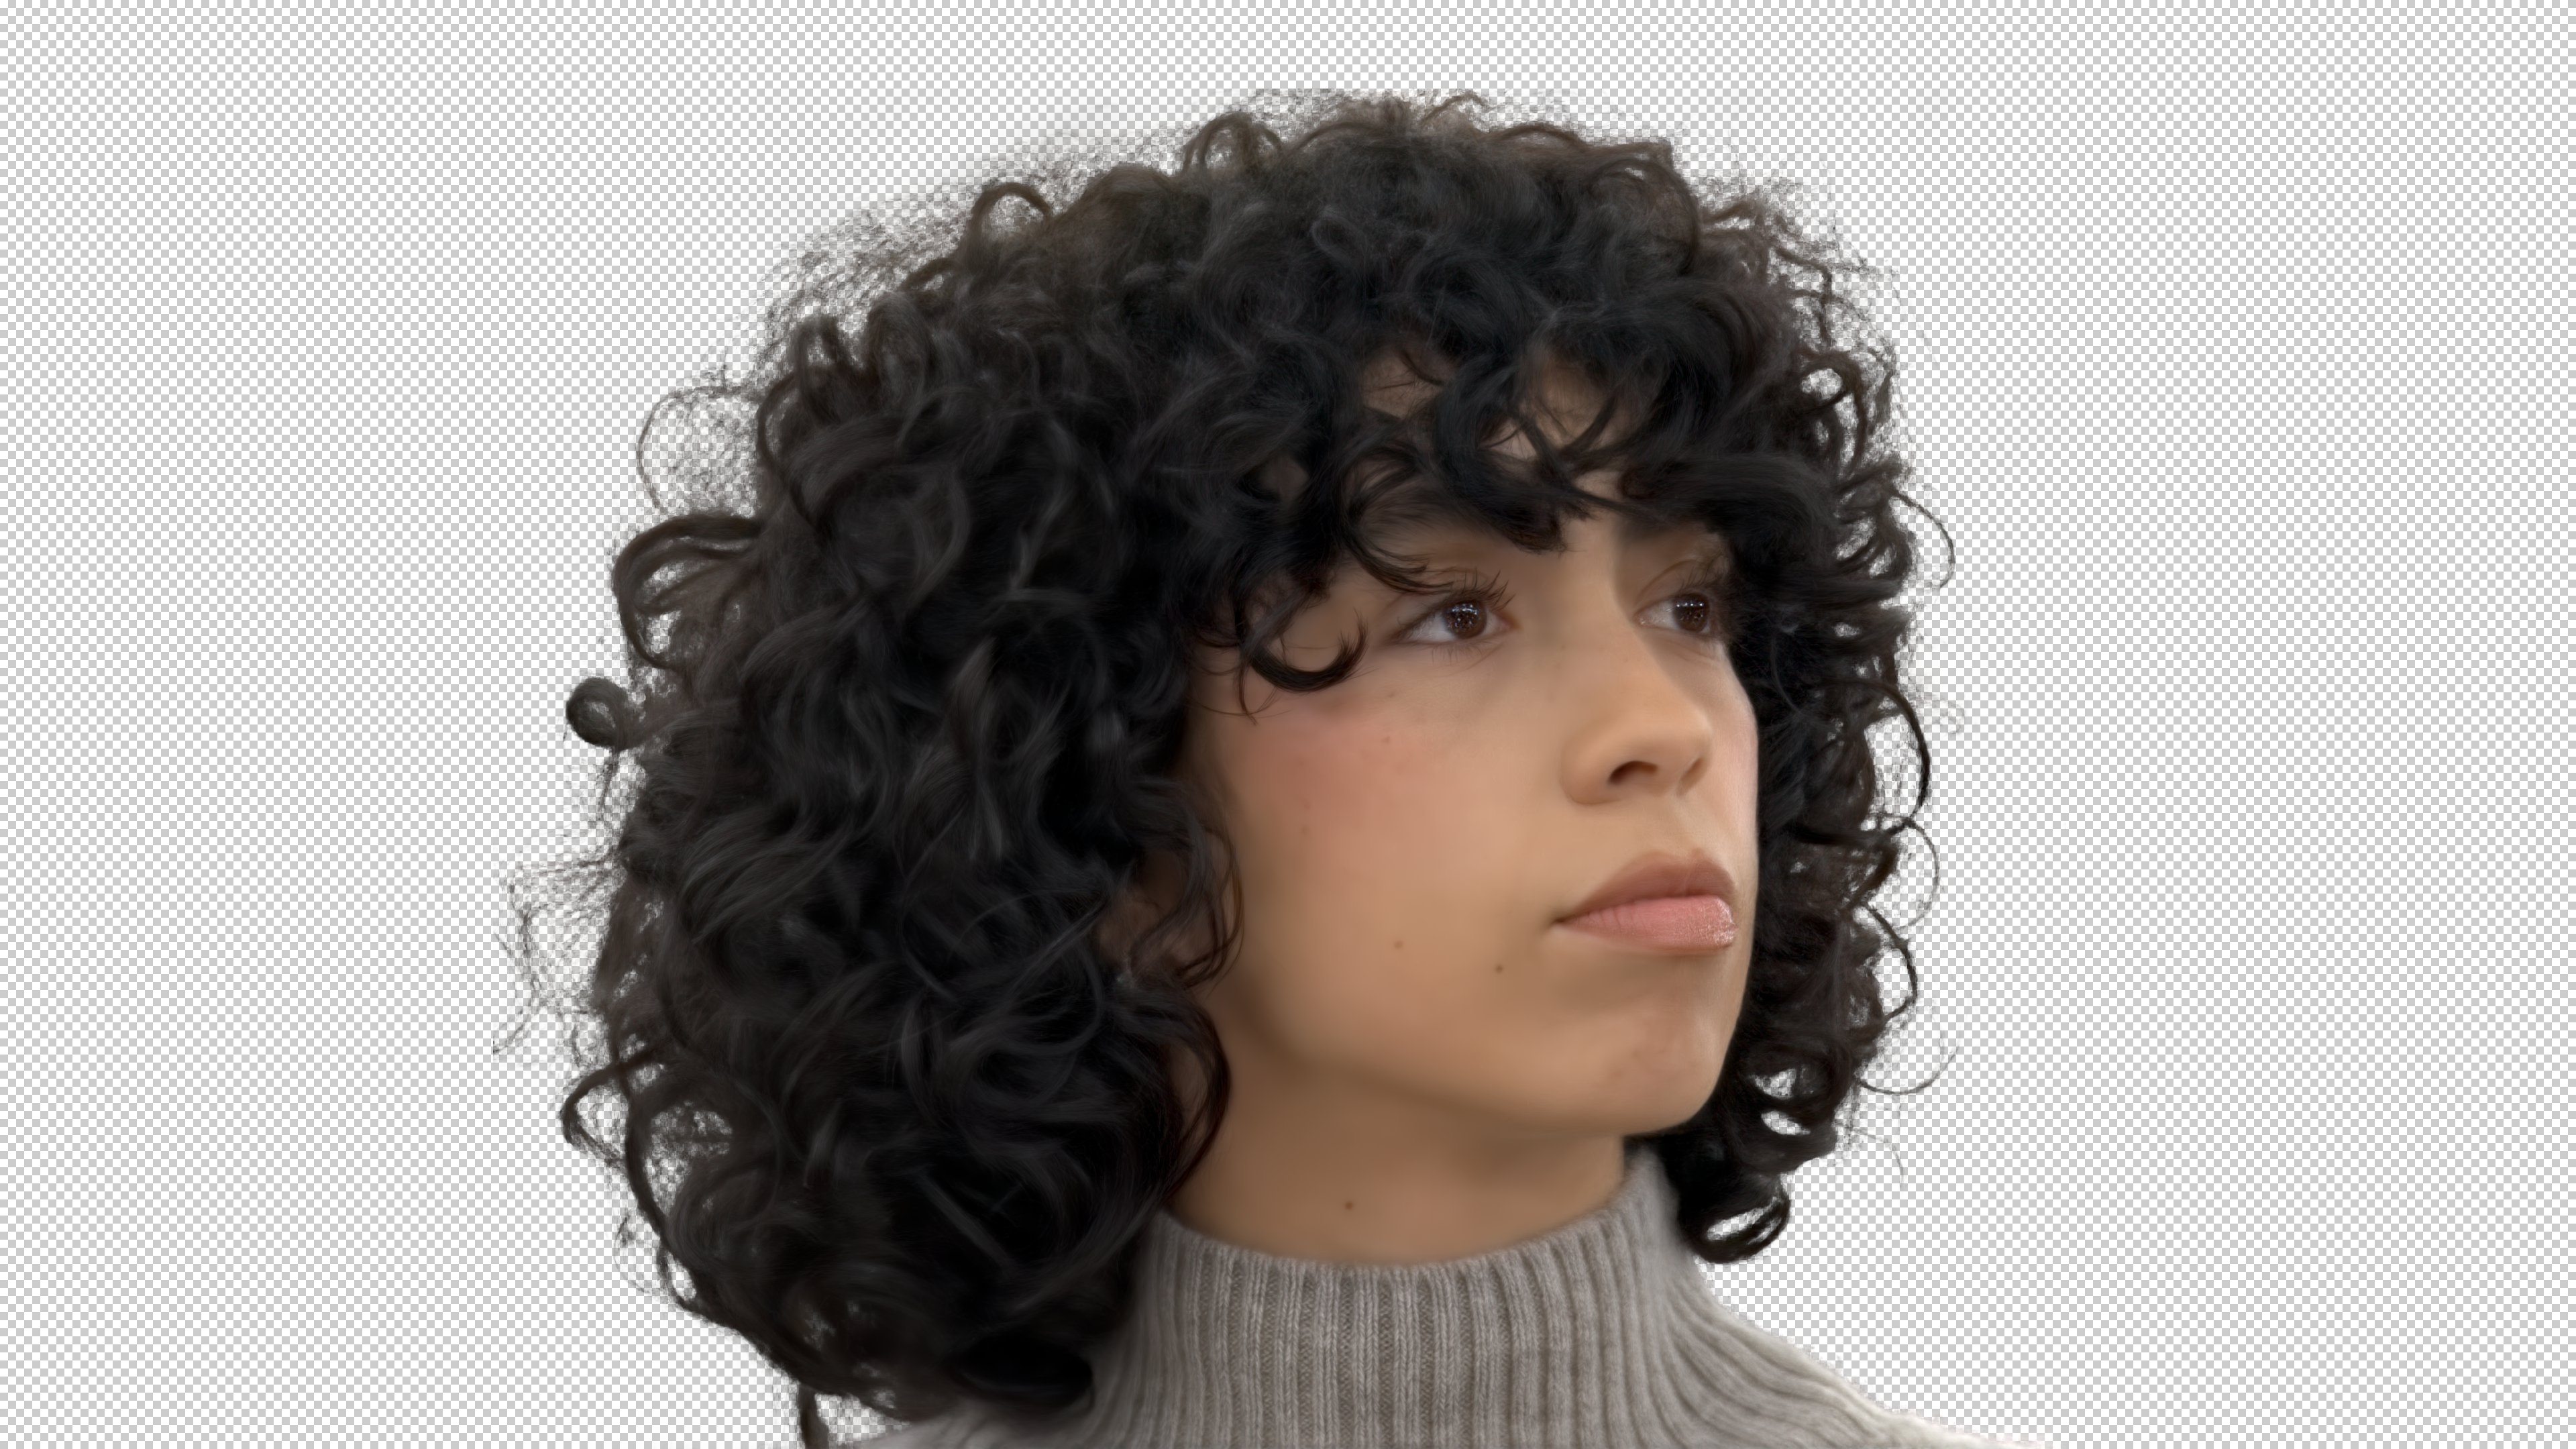}
    \\
    \adjincludegraphics[trim= {0.3\width} {0.3\height} {0.3\width} {0.3\height}, clip, width=\linewidth]{images/main_results/supp/output/cam0000_1114.jpg}
    \end{minipage} \\

    \noalign{\vskip 1mm}   

        \begin{minipage}{0.5\linewidth}
    \centering
    \adjincludegraphics[trim= {0.\width} {0.0\height} {0.\width} {0.0\height}, clip, clip, width=\linewidth]{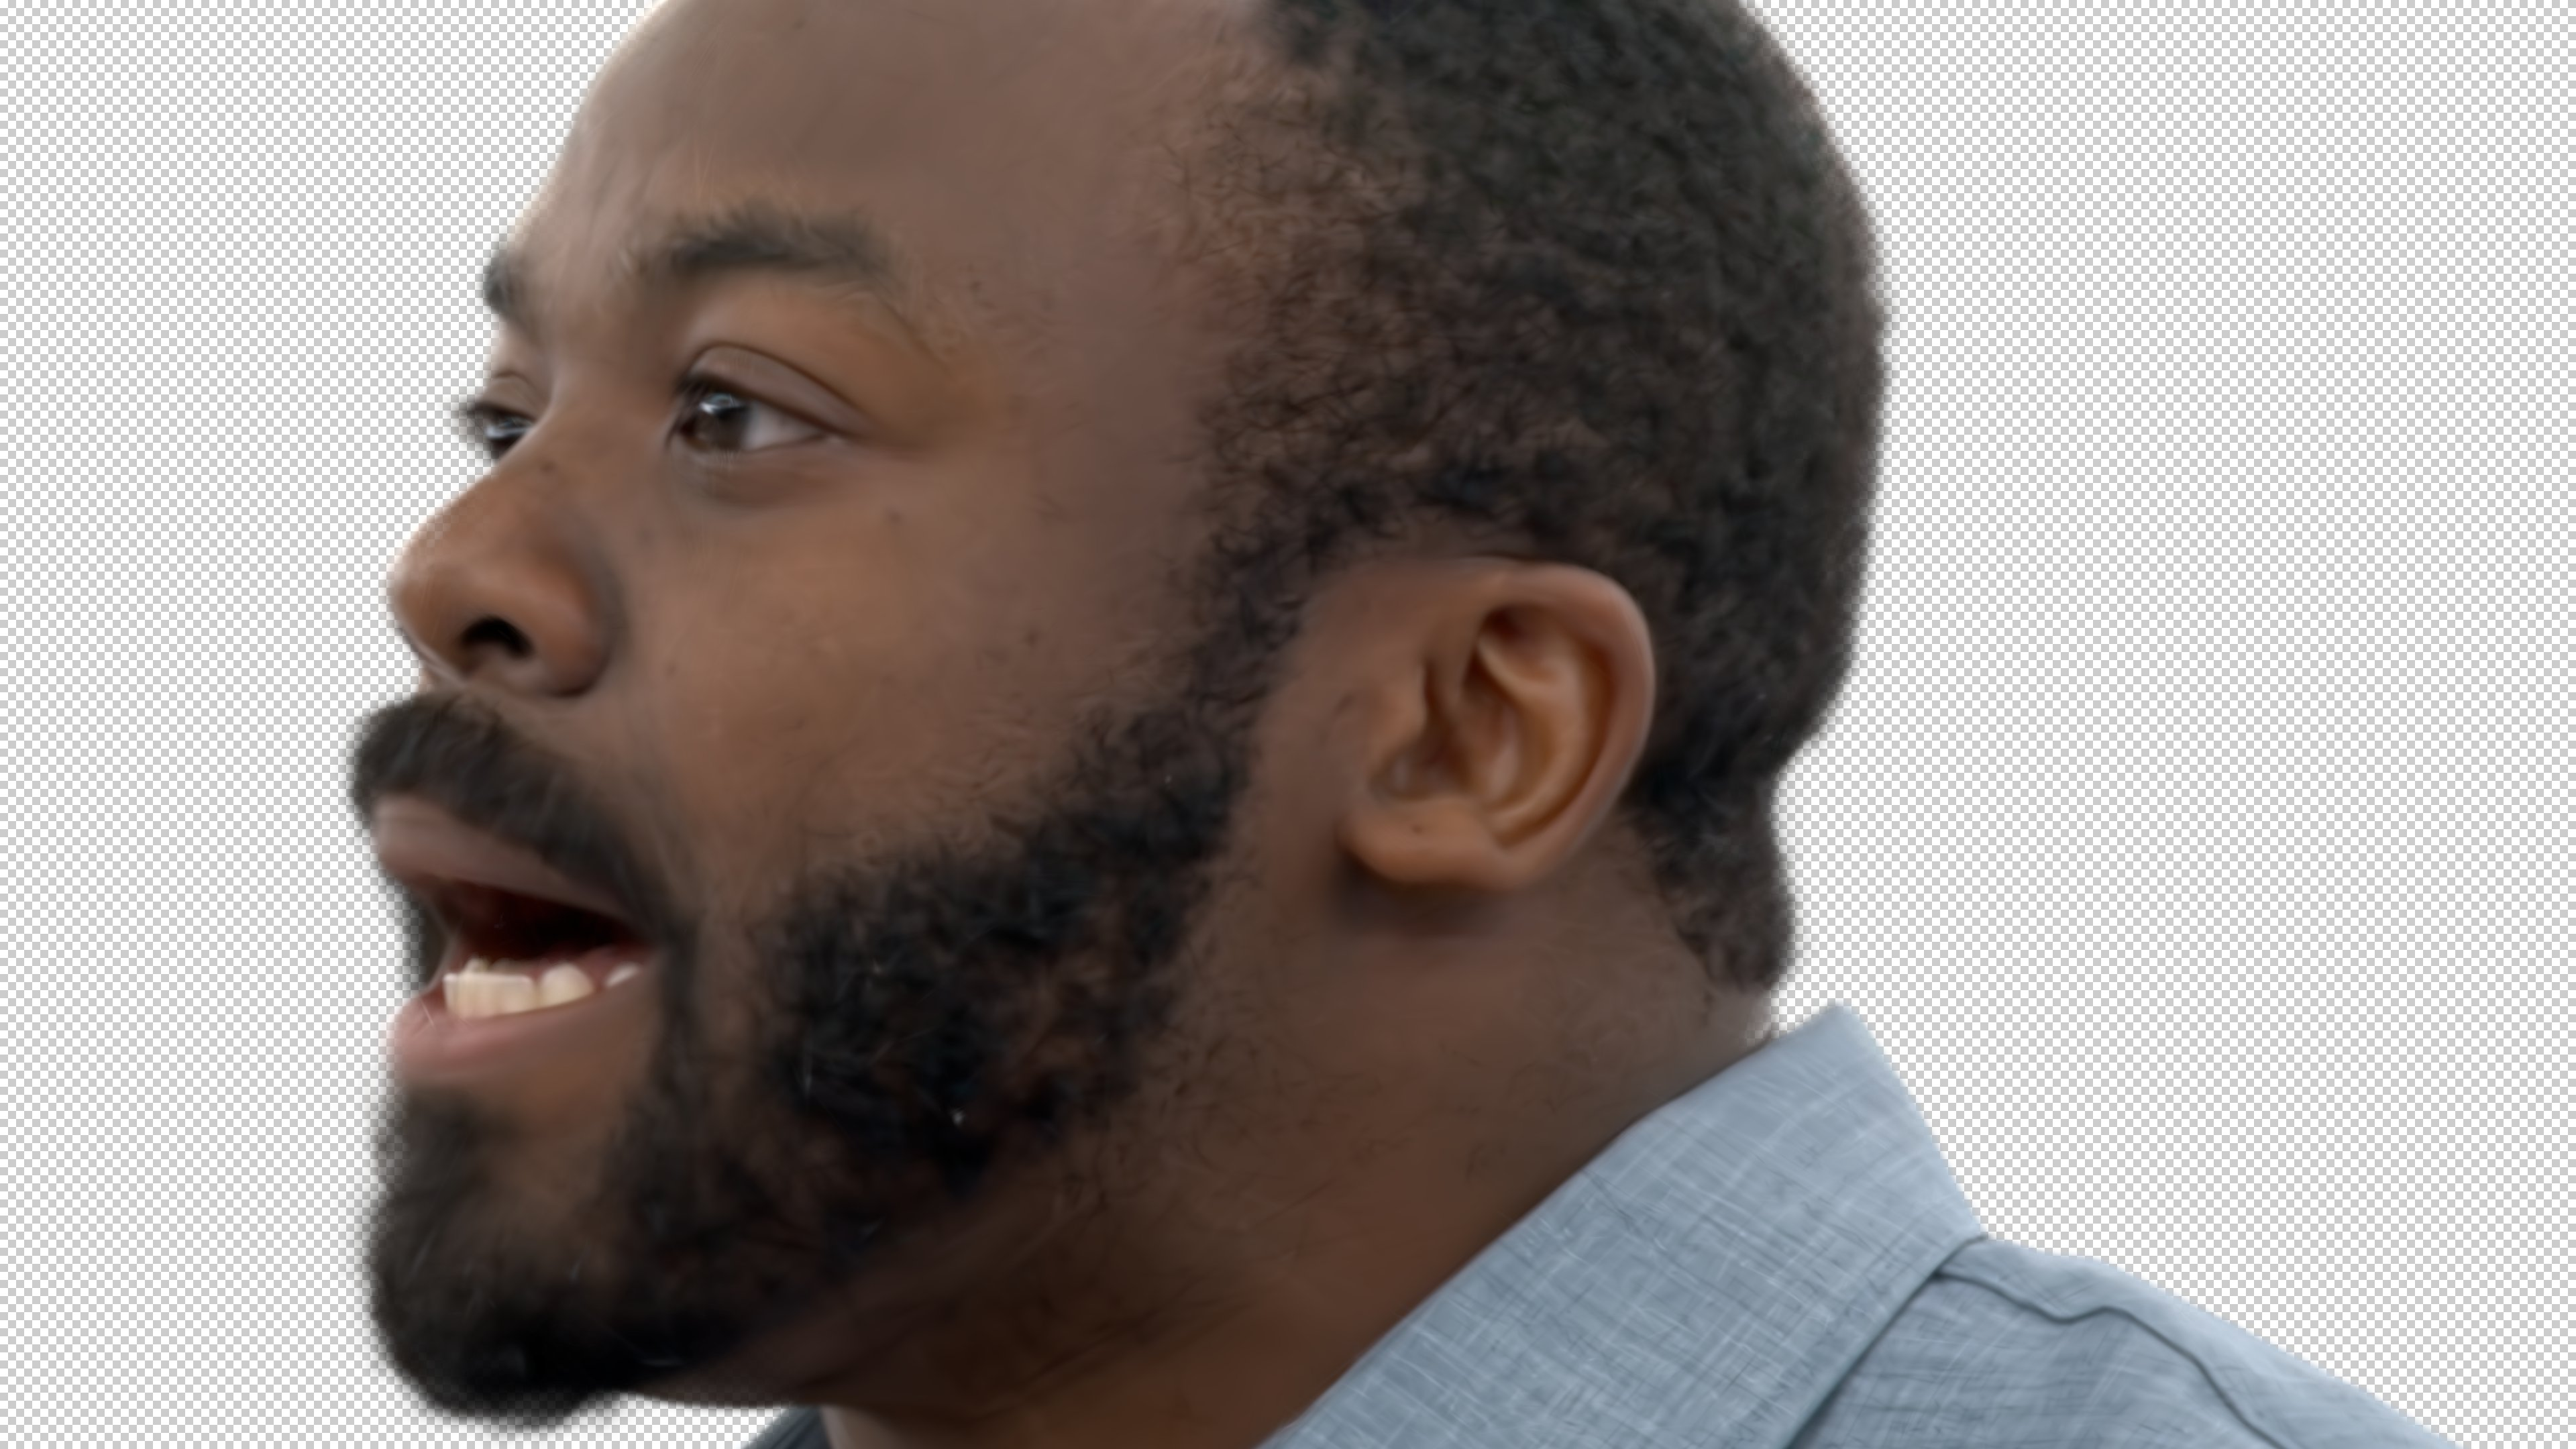}
    \\
    \adjincludegraphics[trim= {0.2\width} {0.25\height} {0.3\width} {0.25\height}, clip, width=\linewidth]{images/main_results/supp/input/cam0000_1161.jpg}
    \end{minipage}

&
    
    \begin{minipage}{0.5\linewidth}
    \centering
    \adjincludegraphics[trim= {0.\width} {0.0\height} {0.\width} {0.0\height}, clip, clip, width=\linewidth]{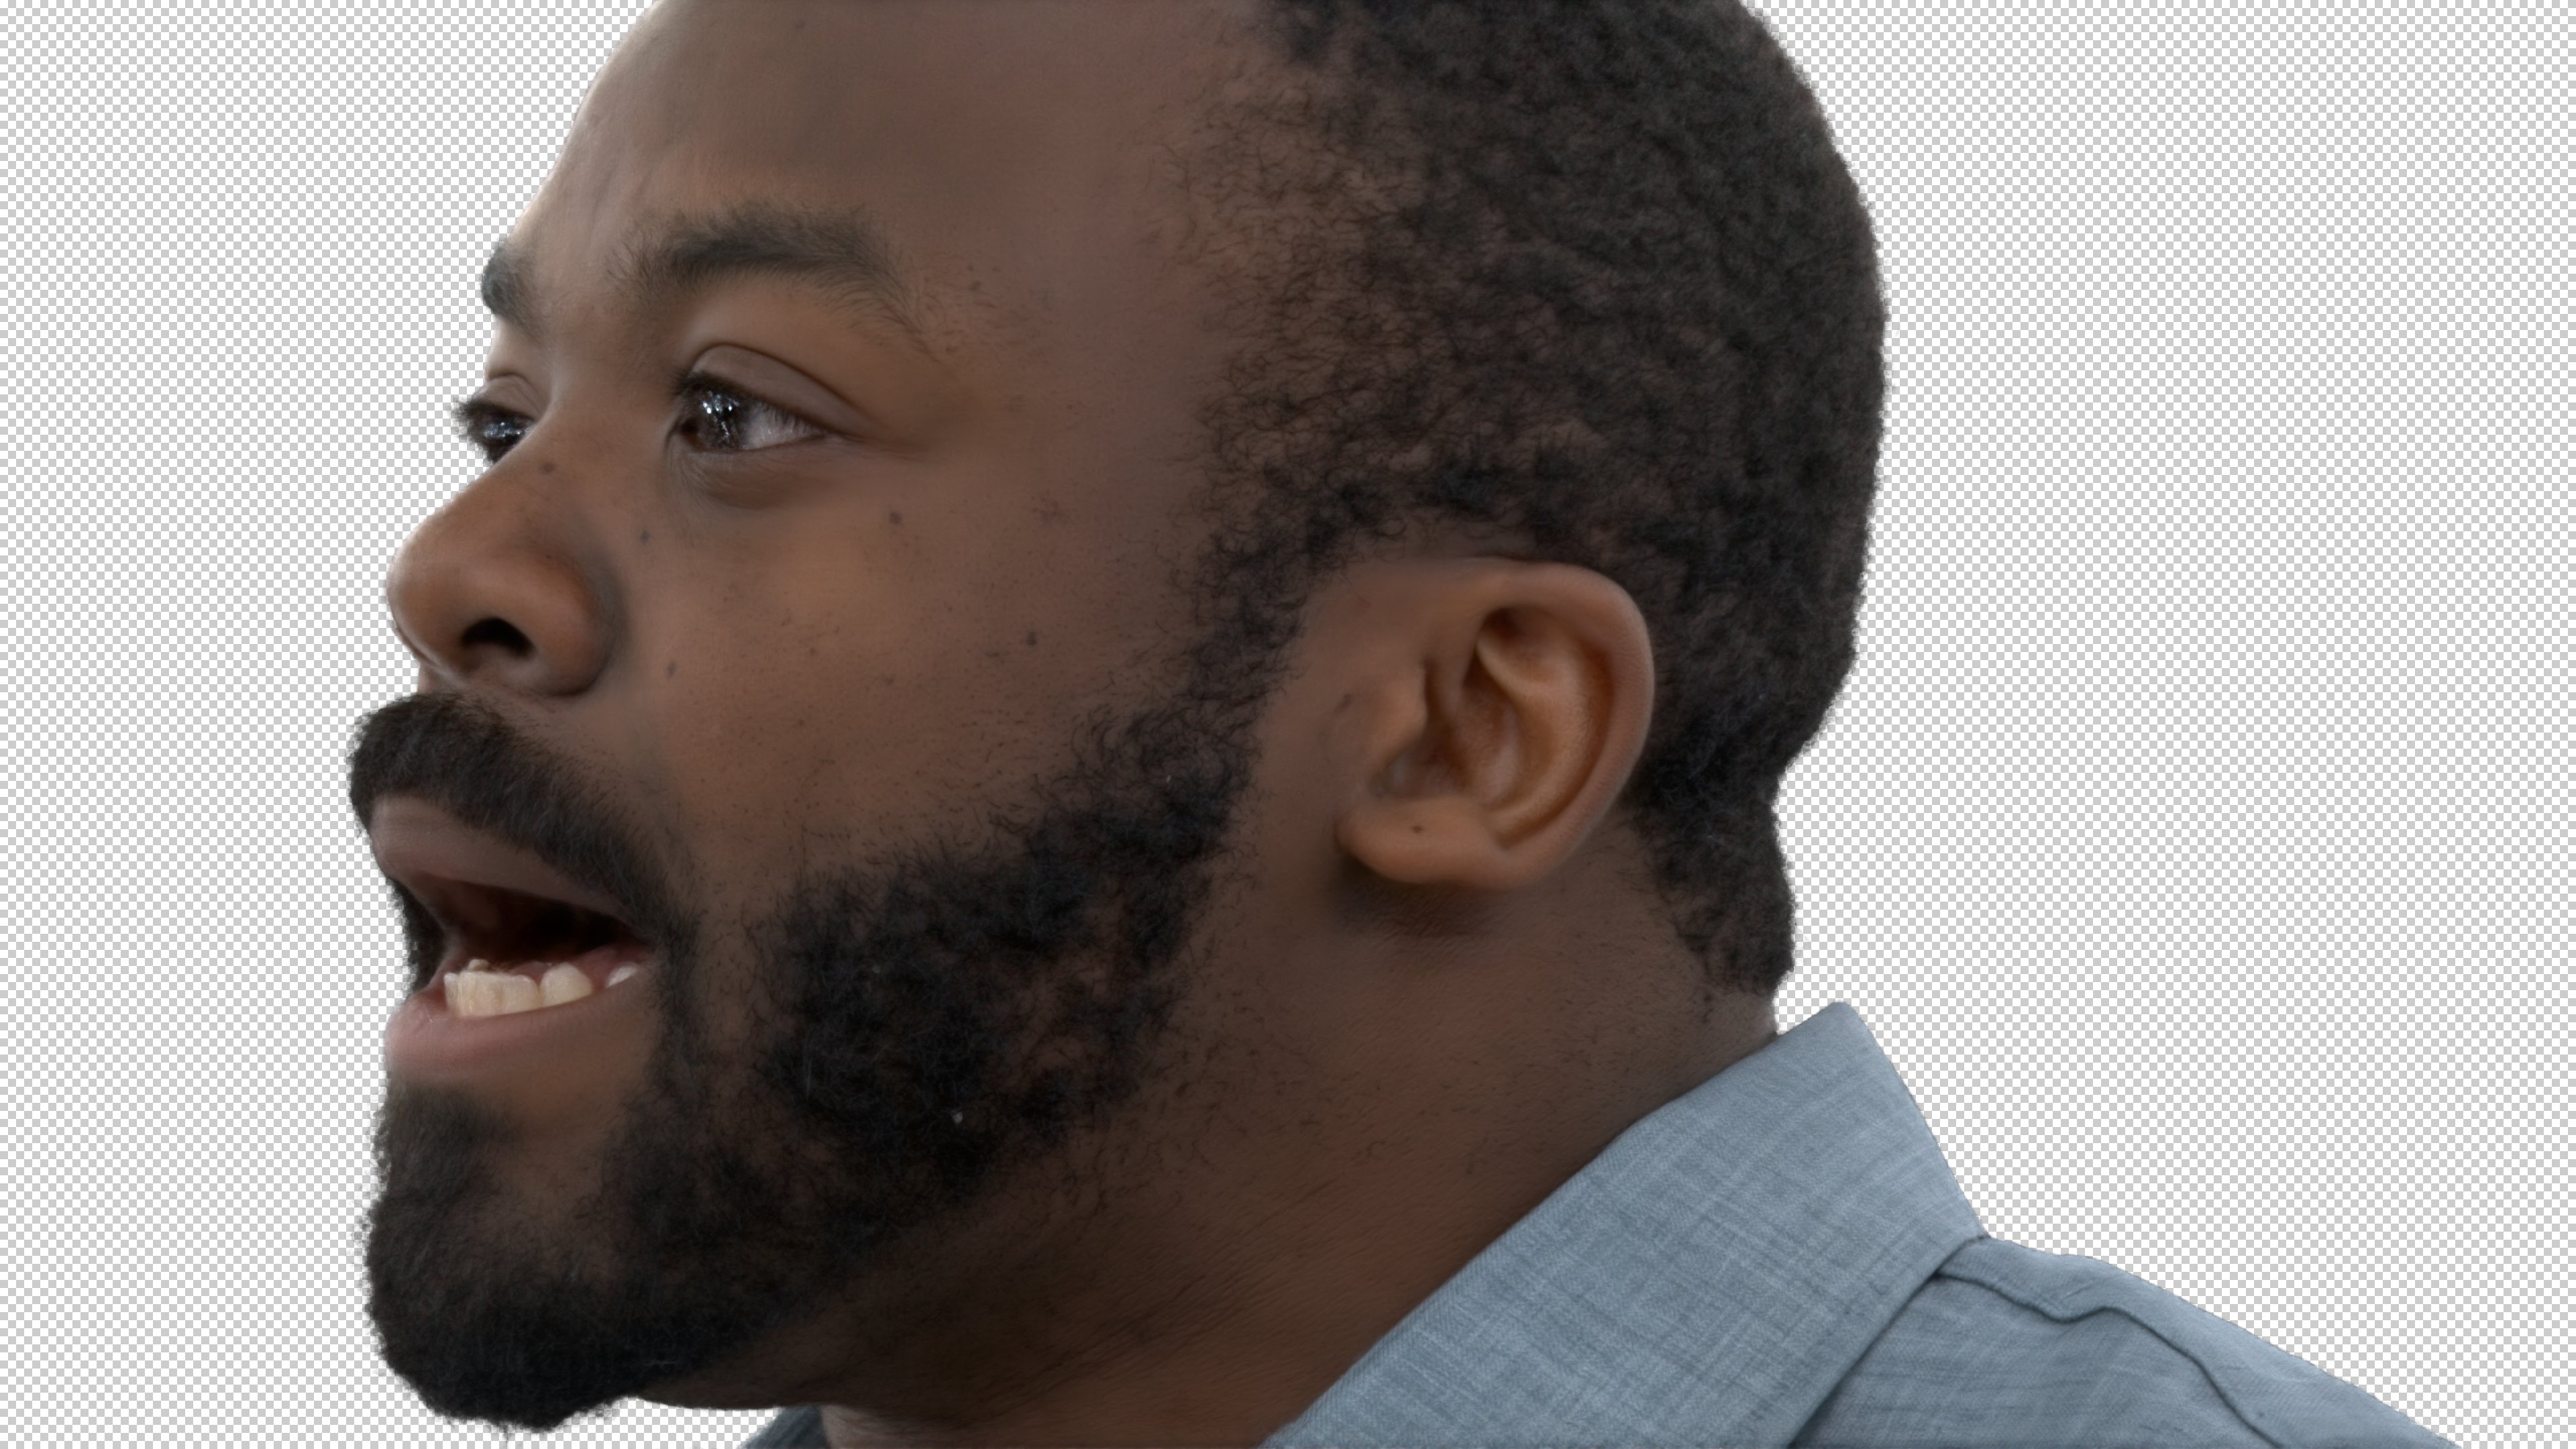}
    \\
    \adjincludegraphics[trim= {0.2\width} {0.25\height} {0.3\width} {0.25\height}, clip, width=\linewidth]{images/main_results/supp/output/cam0000_1161.jpg}
    \end{minipage} \\

\end{tabular}
\caption{Left: our 4DGS reconstruction with insets. Right: final results using our detail enhancement module. We can observe that the Gaussian artifacts are effectively removed and new details added.}
\label{fig:add_results}
\end{figure*}
